# Supplementary material for: Formulas for Continued Fractions. An Automated Guess and Prove Approach
Source: arXiv:1507.04203 ancillary file (2015-07-15)

# Automatic expansion of C-fractions for solutions of Riccati equations via Guessing and Proving.

## The examples from Cuyt *et alii*. Handbook of Continued Fractions for Special Functions

Sébastien Maulat & Bruno Salvy

This worksheet demonstrates the use of the submodule gfun:-ContFrac, for power series solutions of Riccati differential equations :  $y' = p y^2 + q y + r$  with  $p, q, r$  rational in the variable  $z$ .

The first section gives a few examples, and demonstrates how to print some information along the way. A comprehensive list of all the examples from Cuyt *et alii* is then given in the following section.

```
> restart;
> starttime := time();
> with(gfun):

if gfun:-version() < 3.70 then
  error "Old gfun version. Please download the latest version on
  gfun's website, http://perso.ens-lyon.fr/bruno.salvy/software/the-
  gfun-package/."
fi;

with(gfun:-ContFrac):
```

### First examples.

The procedure `expr_to_cfrac` takes as input:

- `expr`: an expression in  $z$
- `y`: a function name
- `z`: a variable name

and optionally :

- a number (the series expansion order)

```
> expr_to_cfrac( exp(z), y, z );
```

$$1 + \frac{z}{1 + \frac{a_1 z}{1 + \frac{\dots}{1 + \frac{a_n z}{1 + \dots}}}}, a_n = \begin{cases} \frac{1}{2(n+1)} & n::\text{even} \\ -\frac{1}{2n} & n::\text{odd} \end{cases} \quad (1.1)$$

The `infolevel` command enables to print details on the computation.

The 'demo' field concerns the main computation lines ; it can be set to 0 or 1.

```
> infolevel[demo] := 1;
```

$$\text{infolevel}_{demo} := 1 \quad (1.2)$$

```
> expr_to_cfrac( tan(z), y, z );
computing series...
... done.
computing a Riccati equation (using a guessing approach)...
... done.
```

$$\left\{ \frac{d}{dz} y(z) - 1 - y(z)^2, y(0) = 0 \right\}$$

```
computing a C-fraction expansion...
... done. (in .524 seconds)
```

$$\frac{z}{1 + \frac{a_1 z^2}{1 + \frac{\dots}{1 + \frac{a_n z^2}{1 + \dots}}}}, a_n = -\frac{1}{(2n-1)(2n+1)} \quad (1.3)$$

```
> infolevel[demo] := 0;
```

$$\text{infolevel}_{demo} := 0 \quad (1.4)$$

More information on how the continued fraction expansion is computed and proved can be printed using the 'gfuncontfrac' information field.

```
> infolevel[gfuncontfrac] := 1;
```

$$\text{infolevel}_{gfuncontfrac} := 1 \quad (1.5)$$

```
> expr_to_cfrac( tan(z), y, z, 20 ):
Guessing a formula
conjecture formula (on 8 coefficients)
```

$$\frac{z}{1 + \frac{a_1 z^2}{1 + \frac{\dots}{1 + \frac{a_n z^2}{1 + \dots}}}}, a_n = -\frac{1}{(2n-1)(2n+1)}$$

```
defining a sequence H(n,z), which relates to convergence.
lemma: the conjecture holds iff there exists an unbounded i(n)
s.t., H(i(n),z) tends to 0.
```

(i.e., their valuations tend to infinity)

```
proving Limit(val(H(n,z)), n = infinity) = infinity:
```

```
- computing a recurrence for H(n,z).
```

(which does not conclude)

$$\dots z^8 H(n) + \dots z^4 H(n+1) + (\dots z^4 + \dots z^2) H(n+2) + \dots H(n+3) + \dots H(n+4) = 0$$

```
- reducing the recurrence order for H(n,z)...
```

```
- ... done.
```

$$\{-z^2 H(n) + (2n+3)^2 H(n+1), H(0) = -z^2\}$$

QED.

```

> infolevel[demo] := 0;
infolevel[gfuncontfrac] := 0;
                                infolevel_demo := 0
                                infolevel_gfuncontfrac := 0

```

(1.6)

## ▼ C-fractions formulas of Riccati solutions in *Cuyt et alii*.

In this section, formulas from the compendium by Cuyt *et alii* (2008) are recovered automatically. All explicit C-fractions solutions of Riccati equations are recovered.

Formulas are stored in a table gfun:-ContFrac:-Cuyt\_Cfrac, which is accessed as follows:

```

> chapter:=11;
                                chapter := 11

```

(2.1)

```

> labels(chapter);
    [1.2, 1.3, 2.2, 2.4, 3.7, 4.5, 4.8, 5.5, 6.4, 6.9, 7.1, 7.2, 7.4]

```

(2.2)

```

> Cuyt_Cfrac[chapter][1.3];
                                e^z

```

(2.3)

In what follows, only the parameters related to the series exponents are given example values.

### ▼ Chapter 11

```

> chapter := 11;
                                chapter := 11

```

(2.1.1)

```

> labels(chapter);
    [1.2, 1.3, 2.2, 2.4, 3.7, 4.5, 4.8, 5.5, 6.4, 6.9, 7.1, 7.2, 7.4]

```

(2.1.2)

```

> N:=20;
                                N := 20

```

(2.1.3)

Generic expansion, with finite series as input.

The order of the series is doubled when the C-fraction coefficients are in  $z^2$ .

```

> for formula in labels(chapter) do

    print( sprintf("%a.%a",chapter,formula) );
    f := Cuyt_Cfrac[chapter][formula];
    print(f);

    if formula in {1.3, 2.2, 7.1, 7.2} then
        S := MultiSeries:-series(f,z,N);
    elif formula = 7.4 then
        S := series(f,z,2*N);
    else
        S := MultiSeries:-series(f,z,2*N);
    fi;

    print( expr_to_cfrac( S, y, z ) );

od:
                                "11.1.2"

```

$$\frac{1}{6} \frac{e^z z^2 - 6 e^z z - z^2 + 12 e^z - 6 z - 12}{e^z z - 2 e^z + z + 2}$$

$$\frac{a_0 z^2}{1 + \frac{\dots}{1 + \frac{a_n z^2}{1 + \dots}}}, a_n = \frac{1}{4 (2 n + 3) (2 n + 5)}$$

"11.1.3"

$$e^z$$

$$1 + \frac{z}{1 + \frac{a_1 z}{1 + \frac{\dots}{1 + \frac{a_n z}{1 + \dots}}}}, a_n = \begin{cases} \frac{1}{2 (n + 1)} & n::even \\ -\frac{1}{2 n} & n::odd \end{cases}$$

"11.2.2"

$$- \frac{\ln(1 + z) - z}{\ln(1 + z)}$$

$$\frac{a_0 z}{1 + \frac{\dots}{1 + \frac{a_n z}{1 + \dots}}}, a_n = \begin{cases} \frac{1}{4} \frac{n + 2}{n + 1} & n::even \\ \frac{1}{4} \frac{n + 1}{n + 2} & n::odd \end{cases}$$

"11.2.4"

$$- \frac{\ln\left(-\frac{1 + z}{z - 1}\right) - 2 z}{\ln\left(-\frac{1 + z}{z - 1}\right)}$$

$$\frac{a_0 z^2}{1 + \frac{\dots}{1 + \frac{a_n z^2}{1 + \dots}}}, a_n = - \frac{(n + 1)^2}{(2 n + 1) (2 n + 3)}$$

"11.3.7"

$$- \frac{\tan(z) - z}{\tan(z)}$$

$$\frac{a_0 z^2}{1 + \frac{\dots}{1 + \frac{a_n z^2}{1 + \dots}}}, a_n = - \frac{1}{(2n+1)(2n+3)}$$

"11.4.5"

$$- \frac{-z \sqrt{-z^2 + 1} + \arcsin(z)}{\arcsin(z)}$$

$$\frac{a_0 z^2}{1 + \frac{\dots}{1 + \frac{a_n z^2}{1 + \dots}}}, a_n = \begin{cases} - \frac{(n+1)(n+2)}{(2n+3)(2n+1)} & n::\text{even} \\ - \frac{(n+1)n}{(2n+3)(2n+1)} & n::\text{odd} \end{cases}$$

"11.4.8"

$$- \frac{\arctan(z) - z}{\arctan(z)}$$

$$\frac{a_0 z^2}{1 + \frac{\dots}{1 + \frac{a_n z^2}{1 + \dots}}}, a_n = \frac{(n+1)^2}{(2n+1)(2n+3)}$$

"11.5.5"

$$- \frac{\tanh(z) - z}{\tanh(z)}$$

$$\frac{a_0 z^2}{1 + \frac{\dots}{1 + \frac{a_n z^2}{1 + \dots}}}, a_n = \frac{1}{(2n+1)(2n+3)}$$

"11.6.4"

$$- \frac{-z \sqrt{z^2 + 1} + \operatorname{arcsinh}(z)}{\operatorname{arcsinh}(z)}$$

$$\frac{a_0 z^2}{1 + \frac{\dots}{1 + \frac{a_n z^2}{1 + \dots}}}, a_n = \begin{cases} \frac{(n+1)(n+2)}{(2n+3)(2n+1)} & n::\text{even} \\ \frac{(n+1)n}{(2n+3)(2n+1)} & n::\text{odd} \end{cases}$$

"11.6.9"

$$\operatorname{arctanh}(z)$$

$$\frac{z}{1 + \frac{a_1 z^2}{1 + \frac{\dots}{1 + \frac{a_n z^2}{1 + \dots}}}}, a_n = -\frac{n^2}{(2n-1)(2n+1)}$$

"11.7.1"

$$-\frac{-\alpha z + (1+z)^\alpha - 1}{(1+z)^\alpha - 1}$$

$$\frac{a_0 z}{1 + \frac{\dots}{1 + \frac{a_n z}{1 + \dots}}}, a_n = \begin{cases} -\frac{1}{4} \frac{-n+2\alpha-2}{n+1} & n::\text{even} \\ \frac{1}{4} \frac{n+2\alpha+1}{n+2} & n::\text{odd} \end{cases}$$

"11.7.2"

$$\frac{(1+z)^\alpha \alpha z - (1+z)^\alpha + 1}{(1+z)^\alpha - 1}$$

$$\frac{a_0 z}{1 + \frac{\dots}{1 + \frac{a_n z}{1 + \dots}}}, a_n = \begin{cases} \frac{1}{4} \frac{n+2\alpha+2}{n+1} & n::\text{even} \\ -\frac{1}{4} \frac{-n+2\alpha-1}{n+2} & n::\text{odd} \end{cases}$$

"11.7.4"

$$\frac{\left( \left( \frac{1 + \frac{1}{z}}{\frac{1}{z} - 1} \right)^\alpha \alpha - \frac{\left( \frac{1 + \frac{1}{z}}{\frac{1}{z} - 1} \right)^\alpha}{z} + \alpha + \frac{1}{z} \right) z}{\left( \frac{1 + \frac{1}{z}}{\frac{1}{z} - 1} \right)^\alpha - 1}$$

$$\frac{a_0 z^2}{1 + \frac{\dots}{1 + \frac{a_n z^2}{1 + \dots}}}, a_n = \frac{(\alpha-1-n)(\alpha+1+n)}{(2n+3)(2n+1)}$$

(2.1.4)

## Chapter 12

```
> chapter := 12;
```

*chapter := 12*

(2.2.1)

```
> N:=25:
```

The parameter  $l$  in formulas (12.6.21) and (12.6.22) is set to a consistent value in order the series to be computed.

```
> vall:=3;
```

*vall := 3*

(2.2.2)

```
> infolevel[gfuncontfrac]:=0;
```

*infolevel<sub>gfuncontfrac</sub> := 0*

(2.2.3)

```
> for formula in labels(chapter) do
```

```
  print( sprintf("%a.%a",chapter,formula) );
  f := Cuyt_Cfrac[chapter][formula]:
```

```
  if formula in {6.21,6.22} then
    print( f, l=vall );
    f := subs( l=vall, f );
  fi;
```

```
  print(expr_to_cfrac( MultiSeries:-series(f,z,N), y, z ) );
```

od:

"12.6.17"

$$\frac{z}{1 + \frac{a_1 z}{1 + \frac{\dots}{1 + \frac{a_n z}{1 + \dots}}}}, a_n = \begin{cases} \frac{1}{2} n & n::\text{even} \\ -a + \frac{1}{2} + \frac{1}{2} n & n::\text{odd} \end{cases}$$

"12.6.21"

$$\begin{aligned} & - \left( \text{pochhammer}(a, l) \left( -e^{-\frac{1}{z}} \left( \frac{1}{z} \right)^a \left( \frac{1}{z} \right)^l \Gamma\left(l + a, \frac{1}{z}\right) \Gamma(a) e^{\frac{1}{z}} a \right. \right. \\ & \quad - e^{-\frac{1}{z}} \left( \frac{1}{z} \right)^a \left( \frac{1}{z} \right)^l \Gamma\left(l + a, \frac{1}{z}\right) \Gamma(a) e^{\frac{1}{z}} l + e^{-\frac{1}{z}} \left( \frac{1}{z} \right)^a \left( \frac{1}{z} \right)^l \Gamma(a + 1 \\ & \quad + l) \Gamma(a) e^{\frac{1}{z}} + e^{-\frac{1}{z}} \left( \frac{1}{z} \right)^{l+a} \Gamma(a + 1 + l) \Gamma\left(a, \frac{1}{z}\right) e^{\frac{1}{z}} \\ & \quad \left. \left. - e^{-\frac{1}{z}} \left( \frac{1}{z} \right)^{l+a} \Gamma(a + 1 + l) \Gamma(a) e^{\frac{1}{z}} - \left( \frac{1}{z} \right)^{l+a} \Gamma(a + 1 + l) \Gamma\left(a, \frac{1}{z}\right) \right) \right) \end{aligned}$$

$$\left/ \left( \left( \frac{1}{z} \right)^l \left( \frac{1}{z} \right)^a e^{-\frac{1}{z}} \left( \frac{1}{z} \right)^{l+a} \Gamma(a+1+l) \right), l=3 \right.$$

$$\frac{z}{1 + \frac{a_1 z}{1 + \frac{\dots}{1 + \frac{a_n z}{1 + \dots}}}}, a_n = \begin{cases} \frac{1}{2} n & n::\text{even} \\ -a - \frac{5}{2} + \frac{1}{2} n & n::\text{odd} \end{cases}$$

"12.6.22"

$$\begin{aligned} & - \left( \left( -\frac{1}{z} \right)^l \left( \frac{\text{pochhammer}(1-a, l) \text{hypergeom}([1, l+1-a], [], -z) e^{-\frac{1}{z}} \left( \frac{1}{z} \right)^a}{z} \right. \right. \\ & + \left( -\frac{1}{z} \right)^{l+1} \text{hypergeom}([1, 1-a], [], -z) e^{-\frac{1}{z}} \left( \frac{1}{z} \right)^a \\ & \left. \left. - \frac{\left( -\frac{1}{z} \right)^{l+1} \Gamma\left(a, \frac{1}{z}\right)}{z} \right) z \right) / \left( \text{pochhammer}(1-a, l) \left( \frac{1}{z} \right)^a e^{-\frac{1}{z}} \left( -\frac{1}{z} \right)^{l+1} \right), l=3 \end{aligned}$$

$$\frac{z}{1 + \frac{a_1 z}{1 + \frac{\dots}{1 + \frac{a_n z}{1 + \dots}}}}, a_n = \begin{cases} \frac{1}{2} n & n::\text{even} \\ -a + \frac{7}{2} + \frac{1}{2} n & n::\text{odd} \end{cases}$$

"12.6.23"

$$a \left( \frac{z}{1 + \frac{a_1 z}{1 + \frac{\dots}{1 + \frac{a_n z}{1 + \dots}}}} \right), a_n = \begin{cases} \frac{1}{2} \frac{n}{(a+n)(a+n-1)} & n::\text{even} \\ -\frac{1}{2} \frac{2a+n-1}{(a+n)(a+n-1)} & n::\text{odd} \end{cases} \quad (2.2.4)$$



In this chapter, one parameter (k) is given a value, and some variable changes are performed for simplicity.

```
> chapter:=13;
                                     chapter := 13
(2.3.1)
```

```
> labels(chapter);
                                     [1.11, 2.20, 3.5, 4.9]
(2.3.2)
```

```
> valk := 3;
                                     valk := 3
(2.3.3)
```

```
> N:=34:
> for formula in labels(chapter) do

  print( sprintf("%a.%a",chapter,formula) );

  f := Cuyt_Cfrac[chapter][formula];

  if formula = 3.5 then  f := subs(k=valk,f);
  elif formula = 4.9 then f := subs(z=z/sqrt(I*Pi),f)
  end if;

  print(f);

  S := MultiSeries:-series(f,z,N);

  print(expr_to_cfrac( S, y, z ));
```

od:

$$\begin{aligned} & \text{"13.1.11"} \\ & \sqrt{\pi} z e^{z^2} \operatorname{erf}(z) \\ & \frac{2 z^2}{1 + \frac{a_1 z^2}{1 + \frac{\dots}{1 + \frac{a_n z^2}{1 + \dots}}}}, a_n = \begin{cases} \frac{2 n}{(-1 + 2 n) (2 n + 1)} & n::\text{even} \\ -\frac{2 n}{(-1 + 2 n) (2 n + 1)} & n::\text{odd} \end{cases} \end{aligned}$$

$$\begin{aligned} & \text{"13.2.20"} \\ & \sqrt{\pi} \operatorname{erfc}\left(\frac{1}{z}\right) e^{\frac{1}{z^2}} z \\ & \frac{z^2}{1 + \frac{a_1 z^2}{1 + \frac{\dots}{1 + \frac{a_n z^2}{1 + \dots}}}}, a_n = \frac{1}{2} n \end{aligned}$$

"13.3.5"

$$-\frac{1}{3} \left( 3 \sqrt{\pi} \operatorname{erf}\left(\frac{1}{z}\right) e^{\frac{1}{z^2}} z^2 - 3 e^{\frac{1}{z^2}} \sqrt{\pi} z^2 + 2 \sqrt{\pi} \operatorname{erf}\left(\frac{1}{z}\right) e^{\frac{1}{z^2}} + 2 z^3 - 2 \sqrt{\pi} e^{\frac{1}{z^2}} + 2 z \right) / \left( z \left( \sqrt{\pi} \operatorname{erf}\left(\frac{1}{z}\right) e^{\frac{1}{z^2}} z^2 - e^{\frac{1}{z^2}} \sqrt{\pi} z^2 + 2 \sqrt{\pi} \operatorname{erf}\left(\frac{1}{z}\right) e^{\frac{1}{z^2}} - 2 \sqrt{\pi} e^{\frac{1}{z^2}} + 2 z \right) \right)$$

$$\frac{1}{2} \frac{z}{1 + \frac{a_1 z^2}{1 + \frac{\dots}{1 + \frac{a_n z^2}{1 + \dots}}}}, a_n = \frac{1}{2} n + \frac{3}{2}$$

"13.4.9"

$$\frac{\left( \operatorname{FresnelC}\left(\frac{z}{\sqrt{I \pi}}\right) + I \operatorname{FresnelS}\left(\frac{z}{\sqrt{I \pi}}\right) \right) e^{-\frac{1}{2} z^2} \sqrt{I \pi}}{z}$$

$$1 - \frac{1}{3} \frac{z^2}{1 + \frac{a_1 z^2}{1 + \frac{\dots}{1 + \frac{a_n z^2}{1 + \dots}}}}, a_n = \begin{cases} -\frac{n}{(2n+3)(2n+1)} & n::\text{even} \\ \frac{n+2}{(2n+3)(2n+1)} & n::\text{odd} \end{cases} \quad (2.3.4)$$

## Chapter 14

```
> chapter := 14;
```

*chapter* := 14 (2.4.1)

```
> N:=20;
```

*N* := 20 (2.4.2)

```
> labels(chapter);
```

[1.16, 1.20, 2.24] (2.4.3)

Parameters n and nu are given example values.

```
> valn := 4;
   valnu := 3/2;
```

*valn* := 4

*valnu* :=  $\frac{3}{2}$  (2.4.4)

```
> for formula in labels(chapter) do
```

```

print( sprintf("%a.%a",chapter,formula) );

f := Cuyt_Cfrac[chapter][formula];
print(f);

if formula = 1.16 then
  S := MultiSeries:-series(f,z,N) assuming nu::real;
elif formula = 1.20 then
  S := MultiSeries:-series(f,z,N) assuming 1-nu > 0;
else
  S := MultiSeries:-series(f,z,N);
fi;

print(expr_to_cfrac( S, y, z ));

```

od:

"14.1.16"

$$e^{\frac{1}{z}} \operatorname{Ei}\left(v, \frac{1}{z}\right)$$

$$\frac{z}{1 + \frac{a_1 z}{1 + \frac{\dots}{1 + \frac{a_n z}{1 + \dots}}}}, a_n = \begin{cases} \frac{1}{2} n & n::\text{even} \\ v - \frac{1}{2} + \frac{1}{2} n & n::\text{odd} \end{cases}$$

"14.1.20"

$$\frac{z \left( z^{v-1} \Gamma(1-v) - \operatorname{Ei}(v, z) \right)}{e^{-z}}$$

$$- \frac{z}{(v-1) \left( 1 + \frac{a_1 z}{1 + \frac{\dots}{1 + \frac{a_n z}{1 + \dots}}} \right)}, a_n =$$

$$\begin{cases} \frac{1}{2} \frac{n}{(-v+n+1)(n-v)} & n::\text{even} \\ -\frac{1}{2} \frac{n-2v+1}{(-v+n+1)(n-v)} & n::\text{odd} \end{cases}$$

"14.2.24"

$$\begin{aligned}
& - \frac{\left( \frac{\operatorname{Ei}\left(-\frac{1}{z}\right) e^{\frac{1}{z}}}{z} - 1 \right) z}{\operatorname{Ei}\left(-\frac{1}{z}\right) e^{\frac{1}{z}}} \\
& -2 - \frac{z}{1 + \frac{a_1 z}{1 + \frac{\dots}{1 + \frac{a_n z}{1 + \dots}}}}, a_n = \begin{cases} 1 + \frac{1}{2} n & n::\text{even} \\ \frac{1}{2} n + \frac{1}{2} & n::\text{odd} \end{cases} \quad (2.4.5)
\end{aligned}$$

## Chapter 15

This chapter has parametrized formulas which are the longest to discover and prove. For this reason, information is printed along the computation.

```
> chapter := 15;
                                chapter := 15
```

(2.5.1)

```
> N:=20;
                                N := 20
```

(2.5.2)

```
> labels(chapter);
                                [3.3, 3.4]
```

(2.5.3)

```
> infolevel[demo]:=1;
infolevel[gfuncontfrac]:=1;
                                infolevel_demo := 1
                                infolevel_gfuncontfrac := 1
```

(2.5.4)

```
> for formula in labels(chapter) do
    print( sprintf("%a.%a",chapter,formula) );
    f := Cuyt_Cfrac[chapter][formula];
    print(f);
    S := series(f,z,N);
    print(expr_to_cfrac( S, y, z ));
od:
                                "15.3.3"
```

$$\frac{\operatorname{hypergeom}([a, b], [c], z)}{\operatorname{hypergeom}([a, b + 1], [c + 1], z)}$$

```
computing series...
... done.
```

computing a Riccati equation (using a guessing approach) ...  
 ... done.

$$\left\{ \frac{d}{dz} y(z) + \frac{z b (a - c) - c (a z - b z - c) y(z) - c^2 y(z)^2}{c (z - 1) z}, y(0) = 1 \right\}$$

computing a C-fraction expansion...

Guessing a formula

conjecture formula (on 16 coefficients)

$$1 + \frac{a_0 z}{1 + \frac{\dots}{1 + \frac{a_n z}{1 + \dots}}}, a_n = \begin{cases} \frac{1}{4} \frac{(2b - 2c - n)(2a + n)}{(c + n)(1 + c + n)} & n::\text{even} \\ \frac{1}{4} \frac{(2b + n + 1)(2a - 2c - n - 1)}{(c + n)(1 + c + n)} & n::\text{odd} \end{cases}$$

defining a sequence  $H(n, z)$ , which relates to convergence.

lemma: the conjecture holds iff there exists an unbounded  $i(n)$  s.t.,  $H(i(n), z)$  tends to 0.

(i.e., their valuations tend to infinity)

proving  $\text{Limit}(\text{val}(H(n, z)), n = \text{infinity}) = \text{infinity}$ :

- computing a recurrence for  $H(n, z)$ .

(which does not conclude)

$$\dots z^4 H(n) + \dots z^2 H(n + 1) + (\dots z^2 + \dots z) H(n + 2) + \dots H(n + 3) + \dots H(n + 4) = 0$$

- computing a P-recurrence for  $H(2*n, z)$  using the rational formulas.

(does not conclude either)

- reducing equation for  $H(2*n, z)$  ...

- ... done.

$$\left\{ - (b + n + 2) (b - c - 1 - n) (a + n + 1) (a - c - n - 2) z^2 H(2n) + (c + 2n + 3)^2 (c + 2n + 2)^2 H(2n + 2), H(0) = - \frac{z^2 a (b + 1) (b - c) (a - c - 1)}{(c + 1)^2} \right\}$$

QED.

... done. (in 275.021 seconds)

$$1 + \frac{a_0 z}{1 + \frac{\dots}{1 + \frac{a_n z}{1 + \dots}}}, a_n = \begin{cases} \frac{1}{4} \frac{(2b - 2c - n)(2a + n)}{(c + n)(1 + c + n)} & n::\text{even} \\ \frac{1}{4} \frac{(2b + n + 1)(2a - 2c - n - 1)}{(c + n)(1 + c + n)} & n::\text{odd} \end{cases}$$

"15.3.4"

$z \text{ hypergeom}([1, a], [c + 1], z)$

computing series...

... done.

computing a Riccati equation (using a guessing approach) ...

... done.

$$\left\{ \frac{d}{dz} y(z) - \frac{-cz - (az - c - z + 1) y(z)}{z (z - 1)}, y(0) = 0 \right\}$$

computing a C-fraction expansion...  
 Guessing a formula  
 conjecture formula (on 16 coefficients)

$$\frac{z}{1 + \frac{a_1 z}{1 + \frac{\dots}{1 + \frac{a_n z}{1 + \dots}}}}, a_n = \begin{cases} \frac{1}{4} \frac{n(2a - 2c - n)}{(c + n)(c + n - 1)} & n::\text{even} \\ -\frac{1}{4} \frac{(2c + n - 1)(2a + n - 1)}{(c + n)(c + n - 1)} & n::\text{odd} \end{cases}$$

defining a sequence  $H(n, z)$ , which relates to convergence.

lemma: the conjecture holds iff there exists an unbounded  $i(n)$  s.t.,  $H(i(n), z)$  tends to 0.

(i.e., their valuations tend to infinity)

proving  $\text{Limit}(\text{val}(H(n, z)), n = \text{infinity}) = \text{infinity}$ :

- computing a recurrence for  $H(n, z)$ .

(which does not conclude)

$$\dots z^4 H(n) + \dots z^2 H(n+1) + (\dots z^2 + \dots z) H(n+2) + \dots H(n+3) + \dots H(n+4) = 0$$

- computing a P-recurrence for  $H(2*n, z)$  using the rational formulas.

(does not conclude either)

- reducing equation for  $H(2*n, z)$ ...

- ... done.

$$\{(n+1)(c+n+1)(a+n+1)(a-c-n-1)z^2 H(2n) + (c+2n+2)^2 (c+2n+1)^2 H(2n+2), H(0) = z^2 a\}$$

QED.

... done. (in 21.190 seconds)

$$\frac{z}{1 + \frac{a_1 z}{1 + \frac{\dots}{1 + \frac{a_n z}{1 + \dots}}}}, a_n = \begin{cases} \frac{1}{4} \frac{n(2a - 2c - n)}{(c + n)(c + n - 1)} & n::\text{even} \\ -\frac{1}{4} \frac{(2c + n - 1)(2a + n - 1)}{(c + n)(c + n - 1)} & n::\text{odd} \end{cases} \quad (2.5.5)$$

> infolevel[demo] := 0;

infolevel[gfuncontfrac] := 0;

infolevel<sub>demo</sub> := 0

infolevel<sub>gfuncontfrac</sub> := 0 (2.5.6)

## Chapter 16

> chapter := 16;

chapter := 16 (2.6.1)

> N:=20;

(2.6.2)

$N := 20$  (2.6.2)

```
> labels(chapter);
```

[1.13, 1.14, 2.4, 3.4, 5.7] (2.6.3)

```
> for formula in labels(chapter) do
```

```
    print( sprintf("%a.%a",chapter,formula) );
```

```
    f := Cuyt_Cfrac[chapter][formula];
```

```
    print(f);
```

```
    S := series(f,z,N);
```

```
    print(expr_to_cfrac( S, y, z ));
```

```
od:
```

"16.1.13"

$$\frac{\text{hypergeom}([a], [b], z)}{\text{hypergeom}([a+1], [b+1], z)}$$

$$1 + \frac{a_0 z}{1 + \frac{\dots}{1 + \frac{a_n z}{1 + \dots}}}, a_n = \begin{cases} \frac{1}{2} \frac{-2b - n + 2a}{(1+n+b)(n+b)} & n::\text{even} \\ \frac{1}{2} \frac{n+1+2a}{(1+n+b)(n+b)} & n::\text{odd} \end{cases}$$

"16.1.14"

$$z \text{ hypergeom}([1], [b+1], z)$$

$$\frac{z}{1 + \frac{a_1 z}{1 + \frac{\dots}{1 + \frac{a_n z}{1 + \dots}}}}, a_n = \begin{cases} \frac{1}{2} \frac{n}{(b+n)(b+n-1)} & n::\text{even} \\ -\frac{1}{2} \frac{2b+n-1}{(b+n)(b+n-1)} & n::\text{odd} \end{cases}$$

"16.2.4"

$$\frac{\text{hypergeom}([a, b], [], z)}{\text{hypergeom}([a, b+1], [], z)}$$

$$1 + \frac{a_0 z}{1 + \frac{\dots}{1 + \frac{a_n z}{1 + \dots}}}, a_n = \begin{cases} -a - \frac{1}{2} n & n::\text{even} \\ -b - \frac{1}{2} - \frac{1}{2} n & n::\text{odd} \end{cases}$$

"16.3.4"

$$\begin{aligned}
 & \frac{\text{hypergeom}([ ], [b], z)}{\text{hypergeom}([ ], [b+1], z)} \\
 & 1 + \frac{a_0 z}{1 + \frac{\dots}{1 + \frac{a_n z}{1 + \dots}}} , a_n = \frac{1}{(n+b)(n+1+b)} \\
 & \text{"16.5.7"} \\
 & e^z \\
 & 1 + \frac{z}{1 + \frac{a_1 z}{1 + \frac{\dots}{1 + \frac{a_n z}{1 + \dots}}}} , a_n = \begin{cases} \frac{1}{2(n+1)} & n::\text{even} \\ -\frac{1}{2n} & n::\text{odd} \end{cases} \quad (2.6.4)
 \end{aligned}$$

## Chapter 17

In this chapter, some functions require to compute the series by hand, as well as the Riccati equation.

The formulas are still produced and proved automatically.

```
> chapter := 17;
                                chapter := 17 (2.7.1)
```

```
> labels(chapter);
[1.37, 1.39, 1.44, 1.46, 2.32, 2.35] (2.7.2)
```

```
> N:=20;
                                N := 20 (2.7.3)
```

```
> for formula in labels(chapter) do
    print( sprintf("%a.%a",chapter,formula) );
    f := subs(n=nn, Cuyt_Cfrac[chapter][formula]);

    if formula = 1.44 then
        lprint("Ad-hoc series computation, and Riccati equation
computation.");
        f := subs(z=z/I, f/exp(-I*Pi));
        print(f);
        f := eval(f, HankelH1 = ContFrac:-myHankelH1);
        f := simplify(f,power,symbolic,exp);
        S := map(simplify,MultiSeries:-series( f, z, N ));

        deq := diff(y(z), z) - (z^2+(2*nu+2)*z^2*y(z)-y(z)^2)
```



```

/z^3:
    print(expr_to_cfrac( S, y, z, riccati = deq ));

elif formula = 1.46 then

    lprint("Ad-hoc series computation.");
    f := subs(z=I*z,f);
    print(f);
    f := eval(f, HankelH2 = ContFrac:-myHankelH2);
    f := simplify(f,power,symbolic,exp);
    S := map(simplify,MultiSeries:-series( f, z, N ));

    print(expr_to_cfrac( S, y, z ));

elif formula = 2.35 then

    print(f);
    S := map(factor,series(f,z,N));
    print(expr_to_cfrac( S, y, z ));

else

    print(f);
    S := MultiSeries:-series( f, z, N );
    print(expr_to_cfrac( S, y, z ));

fi;

od:

```

"17.1.37"

$$\frac{\text{BesselJ}(v+1, z)}{\text{BesselJ}(v, z)}$$

$$\frac{1}{2} \frac{z}{(v+1) \left( 1 + \frac{a_1 z^2}{1 + \frac{\dots}{1 + \frac{a_n z^2}{1 + \dots}}} \right)}, a_n = -\frac{1}{4(n+v)(v+n+1)}$$

"17.1.39"

$$-\frac{1}{2} \frac{2 \text{BesselJ}(nn+1, z) v - z \text{BesselJ}(nn, z) + 2 \text{BesselJ}(nn+1, z)}{\text{BesselJ}(nn+1, z) (v+1)}$$

$$\frac{nn-v}{v+1} + \frac{1}{4} \frac{z^2}{(nn v + nn + 2 v + 2) \left( 1 + \frac{a_1 z^2}{1 + \frac{\dots}{1 + \frac{a_n z^2}{1 + \dots}}} \right)}, a_n$$

$$= \frac{1}{4 (nn + n + 1) (nn + n + 2)}$$

"17.1.44"

"Ad-hoc series computation, and Riccati equation computation."  
"

$$\frac{{}_1z\operatorname{HankelH1}\left(v+1,\frac{1}{z}\right)}{\operatorname{HankelH1}\left(v,\frac{1}{z}\right)}$$

$$\frac{z}{1+\frac{-vz-\frac{1}{2}z}{1+\frac{a_2z}{1+\frac{\dots}{1+\frac{a_nz}{1+\dots}}}}}, a_n = \begin{cases} \frac{1}{2}v + \frac{1}{4} + \frac{1}{4}n & n::\text{even} \\ -\frac{1}{2}v - \frac{1}{2} + \frac{1}{4}n & n::\text{odd} \end{cases}$$

"17.1.46"

"Ad-hoc series computation."

$$\frac{{}_1z\operatorname{HankelH2}\left(v+1,-\frac{1}{z}\right)}{\operatorname{HankelH2}\left(v,-\frac{1}{z}\right)}$$

$$-\frac{z}{1+\frac{-vz-\frac{1}{2}z}{1+\frac{a_2z}{1+\frac{\dots}{1+\frac{a_nz}{1+\dots}}}}}, a_n = \begin{cases} \frac{1}{2}v + \frac{1}{4} + \frac{1}{4}n & n::\text{even} \\ -\frac{1}{2}v - \frac{1}{2} + \frac{1}{4}n & n::\text{odd} \end{cases}$$

"17.2.32"

$$-\frac{1}{2} \frac{2 \operatorname{BesselI}(v+1, z) v - z \operatorname{BesselI}(v, z) + 2 \operatorname{BesselI}(v+1, z)}{\operatorname{BesselI}(v+1, z) (v+1)}$$

$$\frac{1}{4} \frac{z^2}{(v^2 + 3v + 2) \left( 1 + \frac{a_1 z^2}{1 + \frac{\dots}{1 + \frac{a_n z^2}{1 + \dots}}} \right)}, a_n = \frac{1}{4 (v + n + 1) (v + n + 2)}$$

"17.2.35"

$$\frac{1}{2} \frac{1}{-\text{BesselK}\left(v, \frac{1}{z}\right) + \text{BesselK}\left(v+1, \frac{1}{z}\right)} \left( \left( 2 \text{BesselK}\left(v+1, \frac{1}{z}\right) v - \frac{2 \text{BesselK}\left(v+1, \frac{1}{z}\right)}{z} + \frac{2 \text{BesselK}\left(v, \frac{1}{z}\right)}{z} + \text{BesselK}\left(v+1, \frac{1}{z}\right) \right) z \right)$$

$$\frac{a_0 z}{1 + \frac{\dots}{1 + \frac{a_n z}{1 + \dots}}}, a_n = \begin{cases} \frac{1}{2} v + \frac{3}{4} + \frac{1}{4} n & n::\text{even} \\ -\frac{1}{2} v + \frac{1}{4} n & n::\text{odd} \end{cases} \quad (2.7.4)$$

## Chapter 18

```
> chapter := 18;
chapter := 18 (2.8.1)
```

```
> labels(chapter);
[2.16, 2.17, 2.22, 3.4, 4.20] (2.8.2)
```

```
> N:=40;
N := 40 (2.8.3)
```

```
> alpha := 2;
α := 2 (2.8.4)
```

```
> for formula in labels(chapter) do
  print( sprintf("%a.%a",chapter,formula) );
```

```
  f := Cuyt_Cfrac[chapter][formula];
  print(f);
  S := MultiSeries:-series( f, z, N );
  print(expr_to_cfrac( S, y, z ));
```

od:

"18.2.16"

$$\frac{1}{2} \frac{\text{erfc}\left(\frac{1}{2} \frac{\sqrt{2}}{z}\right) z \sqrt{2} \sqrt{\pi}}{e^{-\frac{1}{2z^2}}}$$

$$\frac{z^2}{1 + \frac{a_1 z^2}{1 + \frac{\dots}{1 + \frac{a_n z^2}{1 + \dots}}}}, a_n = n$$

"18.2.17"

$$- \frac{e^{-\frac{1}{2} z^2} z \sqrt{2} + \operatorname{erfc}\left(\frac{1}{2} z \sqrt{2}\right) \sqrt{\pi} - \sqrt{\pi}}{\sqrt{\pi} \left(\operatorname{erfc}\left(\frac{1}{2} z \sqrt{2}\right) - 1\right)}$$

$$\frac{a_0 z^2}{1 + \frac{\dots}{1 + \frac{a_n z^2}{1 + \dots}}}, a_n = \begin{cases} -\frac{n+1}{(2n+1)(2n+3)} & n::\text{even} \\ \frac{n+1}{(2n+1)(2n+3)} & n::\text{odd} \end{cases}$$

"18.2.22"

$$- \frac{1}{2} \frac{\left(\sqrt{2} \sqrt{\pi} e^{\frac{1}{2} z^2} \operatorname{erfc}\left(\frac{1}{2} z \sqrt{2}\right) - \sqrt{2} \sqrt{\pi} e^{\frac{1}{2} z^2} + 2 z\right) \sqrt{2}}{\sqrt{\pi} e^{\frac{1}{2} z^2} \left(\operatorname{erfc}\left(\frac{1}{2} z \sqrt{2}\right) - 1\right)}$$

$$\frac{a_0 z^2}{1 + \frac{\dots}{1 + \frac{a_n z^2}{1 + \dots}}}, a_n = \begin{cases} -\frac{n+1}{(2n+1)(2n+3)} & n::\text{even} \\ \frac{n+1}{(2n+1)(2n+3)} & n::\text{odd} \end{cases}$$

"18.3.4"

$$- \frac{1}{4} \left( \frac{\sqrt{\pi} \operatorname{erf}\left(\frac{1}{2} \frac{\sqrt{2}}{z}\right)}{z^4} + \frac{e^{-\frac{1}{2 z^2}} \sqrt{2}}{z^3} - \frac{\sqrt{\pi}}{z^4} + \frac{6 \sqrt{\pi} \operatorname{erf}\left(\frac{1}{2} \frac{\sqrt{2}}{z}\right)}{z^2} \right. \\ \left. + \frac{5 e^{-\frac{1}{2 z^2}} \sqrt{2}}{z} - \frac{6 \sqrt{\pi}}{z^2} + 3 \sqrt{\pi} \operatorname{erf}\left(\frac{1}{2} \frac{\sqrt{2}}{z}\right) - 3 \sqrt{\pi} \right) / \\ \left( \frac{\sqrt{\pi} \operatorname{erf}\left(\frac{1}{2} \frac{\sqrt{2}}{z}\right)}{z^3} + \frac{e^{-\frac{1}{2 z^2}} \sqrt{2}}{z^2} - \frac{\sqrt{\pi}}{z^3} + \frac{3 \operatorname{erf}\left(\frac{1}{2} \frac{\sqrt{2}}{z}\right) \sqrt{\pi}}{z} \right)$$

$$+ 2 e^{-\frac{1}{2z^2}} \sqrt{2} - \frac{3\sqrt{\pi}}{z} \Bigg)$$

$$\frac{z}{1 + \frac{a_1 z^2}{1 + \frac{\dots}{1 + \frac{a_n z^2}{1 + \dots}}}}, a_n = n + 4$$

"18.4.20"

$$\frac{\left(1 - e^{-\frac{z}{\theta}} \left(1 + \frac{z}{\theta}\right)\right) \theta}{z e^{-\frac{z}{\theta}}}$$

$$\frac{1}{2} \frac{z}{\theta \left(1 + \frac{a_1 z}{1 + \frac{\dots}{1 + \frac{a_n z}{1 + \dots}}}\right)}, a_n = \begin{cases} \frac{1}{2} \frac{n}{\theta (n+2) (n+1)} & n::\text{even} \\ -\frac{1}{2} \frac{n+3}{\theta (n+2) (n+1)} & n::\text{odd} \end{cases} \quad (2.8.5)$$

Next line gives the overall CPU time used for the discovery and proof of all the considered formulas.  
Formulas from other sources are listed below.

```
> time()-starttime;
```

428.776

(1)

## Further formulas.

These are some more examples from other sources.

### logarithmic derivative of Airy function, at infinity

[An indication that this function is of interest appears in an article by the Chudnovsky's in 1991.

We perform a slight linear fractional transformation to remove the first terms, and then discover and prove the formula.

```
> f:=AiryAi(x);
```

$f := \text{AiryAi}(x)$

(3.1.1)

```
> S:=MultiSeries:-asympt(f,x,100):
```

```
> dS:=diff(S,x):
```

```
> dlog:=asympt(dS/S,x,100):
```

```
> St0 := subs(x=1/t^2,dlog):
```

```
> series(t*St0,t,90):
```

```
> St := eval(%,csgn=1):
```

Formula

```
> numtheory[cfrac] (St,t,10,simregular):
> numtheory[cfrac] (% ,t,simregular,quotients) ;
```

$$\left[ -1, \left[ -\frac{1}{4} t^3, 1 \right], \left[ \frac{5}{8} t^3, 1 \right], \left[ \frac{7}{8} t^3, 1 \right], \left[ \frac{11}{8} t^3, 1 \right], \left[ \frac{13}{8} t^3, 1 \right], \left[ \frac{17}{8} t^3, 1 \right], \left[ \frac{19}{8} t^3, 1 \right], \left[ \frac{23}{8} t^3, 1 \right], \left[ \frac{25}{8} t^3, 1 \right], \left[ \frac{29}{8} t^3, 1 \right], \dots \right] \quad (3.1.2)$$

Ad hoc transformation to remove the first terms.

```
> S:=eval( series(1+t^3/4/(1+St),t,90), t=z^(1/3)):
```

The additional argument to `expr_to_cfrac` prevents from too long series to be used in the guessing phase and prevents from memory overuse.

```
> gfun:-ContFrac:-expr_to_cfrac(subs(t=z,S),y,z,10);
```

$$-\frac{5}{8} \frac{z}{1 + \frac{a_1 z}{1 + \frac{\dots}{1 + \frac{a_n z}{1 + \dots}}}}, a_n = \begin{cases} \frac{5}{8} + \frac{3}{8} n & n::even \\ \frac{1}{2} + \frac{3}{8} n & n::odd \end{cases} \quad (3.1.3)$$

## dlmf 4.25.5

```
> f:= exp(2*A*arctan(1/z));
```

$$f := e^{2A \arctan\left(\frac{1}{z}\right)} \quad (3.2.1)$$

```
> A:=2/3;
```

$$A := \frac{2}{3} \quad (3.2.2)$$

```
> g:='g';
```

$$g := g \quad (3.2.3)$$

```
> g:=subs(z=1/z, solve(f=1+2*A/(z-A+g(z)),g(z)));
```

$$g := -\frac{1}{3} \frac{\frac{3 e^{\frac{4}{3} \arctan(z)}}{z} - 2 e^{\frac{4}{3} \arctan(z)} - \frac{3}{z} - 2}{e^{\frac{4}{3} \arctan(z)} - 1} \quad (3.2.4)$$

```
> G := map(normal,series(g,z,40)):
```

```
> gfun:-ContFrac:-expr_to_cfrac(G,y,z,20);
```

$$\frac{13}{27} \frac{z}{1 + \frac{a_1 z^2}{1 + \frac{\dots}{1 + \frac{a_n z^2}{1 + \dots}}}}, a_n = -\frac{1}{9} \frac{(-3n-3+2I)(3n+3+2I)}{(2n+1)(2n+3)} \quad (3.2.5)$$

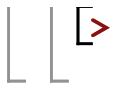

Supplement: Supplementary file 1 [file Cuyt_Riccati_CFracs.pdf]
